# Supplementary material for: Randomized algorithms for matrices and data
Source: arXiv:1104.5557 source file (2011-11-15)
Supplement: Supplementary file 1 [file appendix.tex]

%%\section{Misc stuff}
